# Supplementary material for: Small Decision Trees for MDPs with Deductive Synthesis
Source: arXiv:2501.10126 source file (2025-05-22)
Supplement: Supplementary file 1 [file appendix-q2.tex]

\begin{tabular}{l r@{\hskip 12pt}rrr@{\hskip 12pt}rrr}
\toprule
\multirow{2}{*}{model} & &
\multicolumn{3}{c@{\hskip 12pt}}{\dtmap} &
\multicolumn{3}{c}{\dtcontrol}\\
\cmidrule(lr{1.75em}){3-5}\cmidrule(lr){6-8}
& choices & time & depth & nodes & time & depth & nodes \\
\midrule
lake-4 & 64 & ${<}1$ & 4 & \bf 8 & ${<}1$ & 5 & 10 \\
lake-8 & 256 & ${<}1$ & 6 & \bf 38 & ${<}1$ & 8 & 40 \\
lake-12 & 576 & 4.1 & 7 & \bf 70 & ${<}1$ & 12 & 73 \\
traffic & 722 & 10.6 & 6 & 34 & ${<}1$ & 12 & \bf 32 \\
3d & 750 & ${<}1$ & 3 & \bf 6 & ${<}1$ & 10 & 68 \\
sys-tree & 1024 & 2.7 & 7 & 35 & ${<}1$ & 7 & \bf 12 \\
blackjack & 1066 & ${<}1$ & 4 & 10 & ${<}1$ & 7 & \bf 8 \\
sys-1 & 2304 & 150.2 & 8 & 97 & ${<}1$ & 8 & \bf 76 \\
sys-2 & 2304 & 42.6 & 8 & 67 & ${<}1$ & 8 & \bf 41 \\
pacman & 2951 & 6.2 & 5 & \bf 23 & ${<}1$ & 14 & 183 \\
\cmidrule(lr){1-8}
wlan & 4189 & TO & ${>}$5 & - & ${<}1$ & 11 & \bf 159 \\
ij & 5120 & TO & ${>}$7 & - & ${<}1$ & 10 & \bf 645 \\
firewire & 5515 & 19.3 & 5 & \bf 23 & ${<}1$ & 9 & 69 \\
pnueli & 6457 & 4.4 & 6 & \bf 59 & ${<}1$ & 15 & 857 \\
csma & 7988 & TO & ${>}$5 & - & ${<}1$ & 9 & 54 \\
maze-7 & 8156 & TO & ${>}$6 & - & ${<}1$ & 14 & 280 \\
consensus & 9232 & 14.0 & 5 & \bf 22 & ${<}1$ & 9 & 51 \\
inventory & 10100 & 1.5 & 4 & \bf 14 & ${<}1$ & 6 & \bf 14 \\
resource & 10571 & ${<}1$ & 3 & \bf 7 & ${<}1$ & 16 & 248 \\
philos & 10932 & 11.8 & 6 & \bf 41 & ${<}1$ & 16 & 946 \\
rabin & 15388 & TO & ${>}$5 & - & ${<}1$ & 21 & 154 \\
tictactoe & 21816 & TO & ${>}$5 & - & 1.4 & 14 & 1170 \\
\bottomrule
\end{tabular}
